# Supplementary material for: The Bayesian Sorting Hat: A Decision-Theoretic Approach to Size-Constrained Clustering
Source: arXiv:1710.06047 ancillary file (2017-10-17)
Supplement: Supplementary file 1 [file Sorting_Hat_Supplement_A.pdf]

# SUPPLEMENT A: THE BAYESIAN SORTING HAT

By Justin D. Silverman and Rachel Silverman

CONTENTS

1 Extended Simulation Methods and Results . . . . . . . . . . . . . . 1
1.1 Data Generation . . . . . . . . . . . . . . . . . . . . . . . . . 1
1.2 Results for Equal Group Sizes . . . . . . . . . . . . . . . . . . . 3
1.3 Results for Unequal Group Sizes . . . . . . . . . . . . . . . . . 4
2 Sorting Hat Survey Questions and Associated Priors . . . . . . . . 7
References . . . . . . . . . . . . . . . . . . . . . . . . . . . . . . . 9

## 1. Extended Simulation Methods and Results.

1.1. *Data Generation.* We simulated two datasets consisting of 20 respondents from 3 clusters responding to 10 questions each with 3 possible answers. The first simulated dataset consisted of nearly balanced clusters with the true cluster composition given by the proportions (0.35,0.35,0.30). The second simulated dataset consisted of uneven cluster sizes with the true cluster composition given by the proportions (0.40, 0.35, 0.25).

Datasets were simulated through the categorical mixture model specified in Section 2.3. Specifically both simulated datasets had the same $\alpha$ and $\beta$ parameter settings given in Tables S1 and S2 respectively. In order to ensure there was clustering of the simulated $\theta$ parameters by clusters, we specified a different $\alpha$ for each group. The code required to reproduce our simulations and analysis can be found in Supplement B.

| Respondent | Cluster 1 | Cluster 2 | Cluster 3 |
|---|---|---|---|
| 1 | 1 | 7 | 1 |
| 2 | 7 | 1 | 1 |
| 3 | 7 | 1 | 1 |
| 4 | 7 | 1 | 1 |
| 5 | 1 | 7 | 1 |
| 6 | 7 | 1 | 1 |
| 7 | 1 | 7 | 1 |
| 8 | 1 | 1 | 7 |
| 9 | 1 | 7 | 1 |
| 10 | 1 | 1 | 7 |
| 11 | 7 | 1 | 1 |
| 12 | 7 | 1 | 1 |
| 13 | 1 | 1 | 7 |
| 14 | 7 | 1 | 1 |
| 15 | 1 | 7 | 1 |
| 16 | 1 | 1 | 7 |
| 17 | 1 | 7 | 1 |
| 18 | 7 | 1 | 1 |
| 19 | 1 | 1 | 7 |
| 20 | 1 | 7 | 1 |

TABLE S1

*Chosen $\alpha_n$ hyper-parameters for each simulated respondent*

| Questions | Response | Cluster 1 | Cluster 2 | Cluster 3 |
|---|---|---|---|---|
| 1 | 1 | 1 | 1 | 7 |
| 1 | 2 | 1 | 7 | 1 |
| 1 | 3 | 7 | 1 | 1 |
| 2 | 1 | 8 | 1 | 1 |
| 2 | 2 | 1 | 1 | 8 |
| 2 | 3 | 1 | 5 | 1 |
| 3 | 1 | 2 | 1 | 5 |
| 3 | 2 | 1 | 5 | 2 |
| 3 | 3 | 5 | 1 | 1 |
| 4 | 1 | 5 | 1 | 7 |
| 4 | 2 | 1 | 1 | 5 |
| 4 | 3 | 5 | 8 | 1 |
| 5 | 1 | 6 | 1 | 5 |
| 5 | 2 | 1 | 8 | 2 |
| 5 | 3 | 5 | 1 | 1 |
| 6 | 1 | 6 | 1 | 1 |
| 6 | 2 | 1 | 1 | 5 |
| 6 | 3 | 1 | 8 | 1 |
| 7 | 1 | 1 | 1 | 5 |
| 7 | 2 | 2 | 5 | 1 |
| 7 | 3 | 5 | 1 | 1 |
| 8 | 1 | 5 | 1 | 1 |
| 8 | 2 | 1 | 1 | 5 |
| 8 | 3 | 5 | 8 | 1 |
| 9 | 1 | 1 | 1 | 5 |
| 9 | 2 | 7 | 1 | 1 |
| 9 | 3 | 1 | 10 | 1 |
| 10 | 1 | 5 | 1 | 1 |
| 10 | 2 | 1 | 1 | 5 |
| 10 | 3 | 1 | 8 | 1 |

Table S2

*Chosen $\beta_{kq}$ hyper-parameters for each possible response to each question ($q$) by cluster ($k$).*

1.2. *Results for Equal Group Sizes.* The posterior distribution for $\theta$ for the case of equal group sizes is shown in Figure 1.

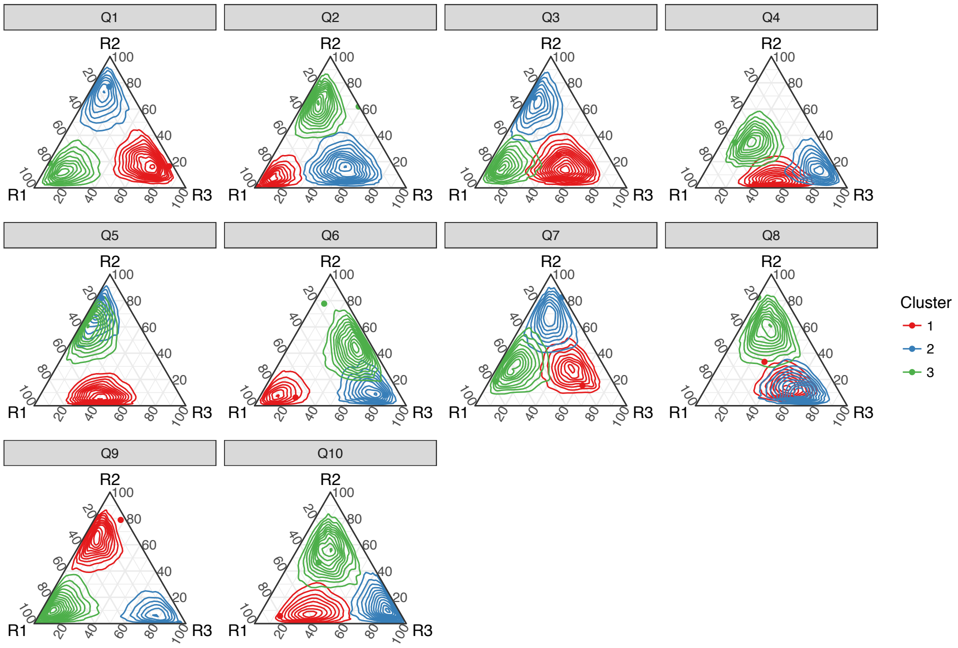


Fig S1. *Posterior distributions for $\phi$ on simulated data with equal group sizes places regions of highest posterior probability near the true simulated values for $\phi$. Posterior distributions for the composition of prototypical responses (R1-R3) for each cluster for each question (Q1-Q9) in a survey are shown using ternary diagrams with kernel density estimates. Kernel density estimates were calculated using the function* stat_density_tern *from the R package* **ggtern** *with default parameters. Points represents the true simulated value of $\phi$ for each group.*

### 1.3. *Results for Unequal Group Sizes.*

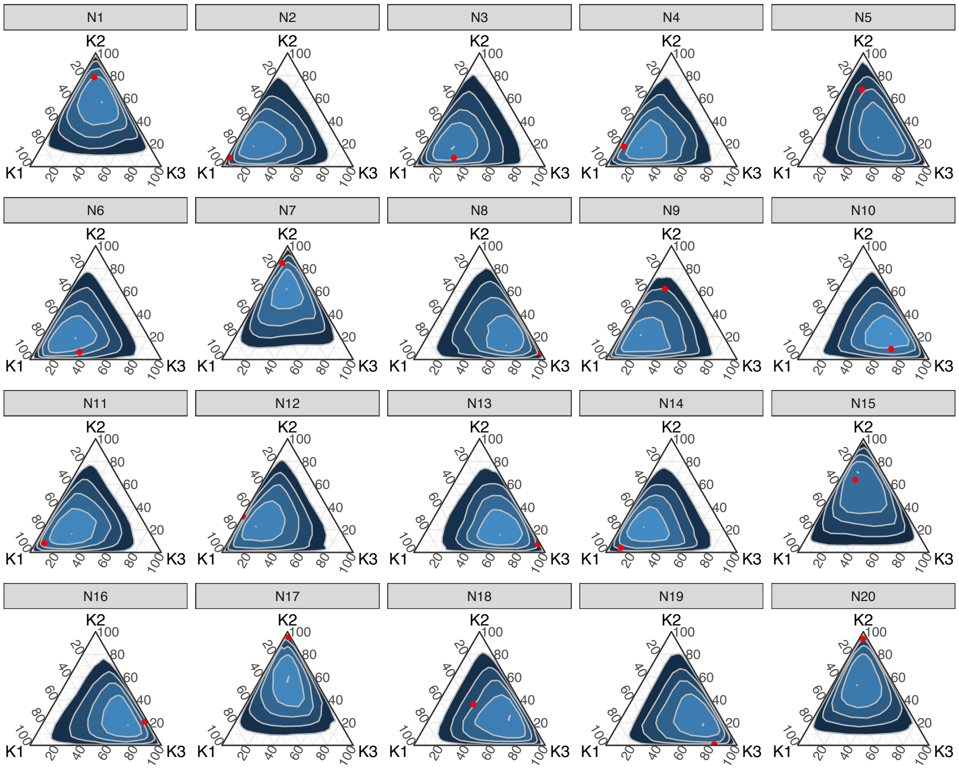


Fig S2. *Posterior distributions for $\theta$ on simulated data with unequal group sizes places regions of highest posterior probability near the true simulated values for $\theta$. Posterior distributions for the composition of 20 respondents (N1-N20) among 3 clusters (K1-K3) are shown using ternary diagrams with kernel density estimates. Kernel density estimates were calculated using the function* stat_density_tern *from the R package* **ggtern** *with the parameter* bins=5. *Red dots represents the true simulated value of $\theta$ for each respondent.*

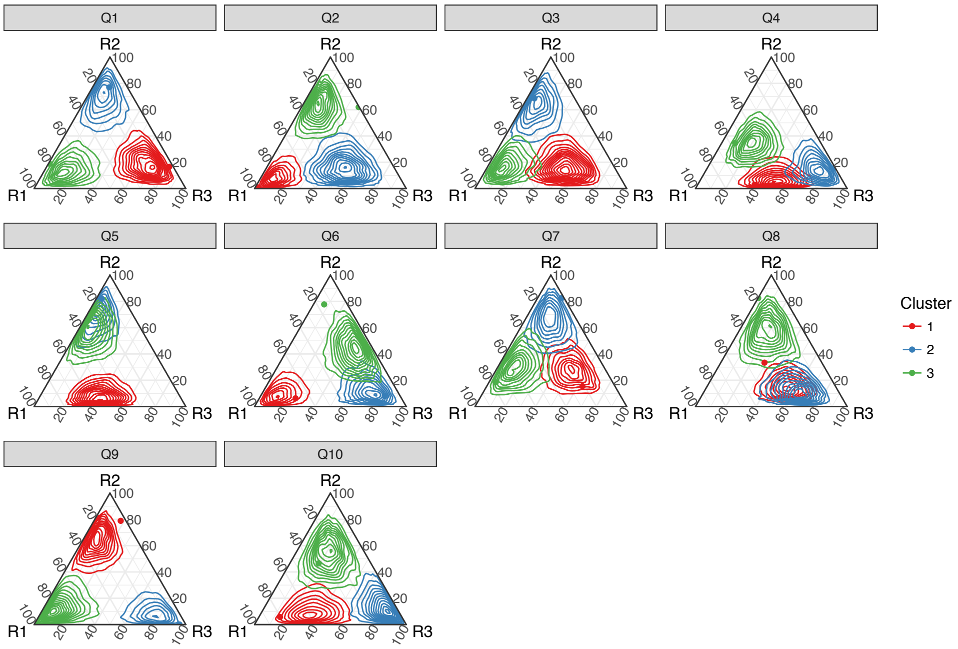


Fig S3. *Posterior distributions for $\phi$ on simulated data with unequal group sizes places regions of highest posterior probability near the true simulated values for $\phi$. Posterior distributions for the composition of prototypical responses (R1-R3) for each cluster for each question (Q1-Q9) in a survey are shown using ternary diagrams with kernel density estimates. Kernel density estimates were calculated using the function* stat_density_tern *from the R package* **ggtern** *with default parameters. Points represents the true simulated value of $\phi$ for each group.*

**2. Sorting Hat Survey Questions and Associated Priors.** Of the 8 questions on the survey, questions 1 through 7 were based on the Sorting Hat quiz available on the Pottermore website (Rowling) while question 8 was of our own design.

1. Moon or Stars?
   (a) Moon
   (b) Stars
2. Which road tempts you most?
   (a) Wide, sunny, grassy lane
   (b) Narrow, dark, lantern-lit alley
   (c) Twisting, leaf strewn path through woods
   (d) Cobbled street lined with ancient buildings
3. Given the choice, would you rather invent a potion that would guarantee you...
   (a) Love
   (b) Glory
   (c) Wisdom
   (d) Power
4. What kind of instrument most pleases your ear?
   (a) Violin
   (b) Trumpet
   (c) Piano
   (d) Drum
5. If you were attending Hogwarts, which pet would you choose to take with you?
   (a) Tabby Cat
   (b) Siamese Cat
   (c) Ginger Cat
   (d) Black Cat
   (e) White Cat
   (f) Tawny Owl
   (g) Screech Owl

   (h) Brown Owl
   (i) Snowy Owl
   (j) Barn Owl
   (k) Common Toad
   (l) Natterjack Toad
   (m) Dragon Toad
   (n) Harlequin Toad
   (o) Three Toes Tree Toad

6. If you would have any power, which would you choose?
   (a) The power to read minds
   (b) The power of invisibility
   (c) The power of superhuman strength
   (d) The power to speak to animals
   (e) The power to change the past
   (f) The power to change you appearance at will
7. Which would you rather be?
   (a) Envied
   (b) Imitated
   (c) Trusted
   (d) Praised
   (e) Liked
   (f) Feared
8. Six or a half dozen?
   (a) Six
   (b) Half dozen

Due to small sample size, we felt it necessary to reduce the possible responses for question 5. To do this we consolidated responses to three categories as follows:

5. If you were attending Hogwarts, which pet would you choose to take with you?
   (a) Cat
   (b) Owl

(c) Toad

It is this reduced version of the question that we placed a prior on as shown in Supplementary Table S3.

| Question | Response | Gryffindor | Slytherin | Ravenclaw | Hufflepuff |
|---|---|---|---|---|---|
| 1 | a | 3.00 | 7.00 | 7.00 | 3.00 |
| 1 | b | 7.00 | 3.00 | 3.00 | 7.00 |
| 2 | a | 2.00 | 2.00 | 1.00 | 4.00 |
| 2 | b | 2.00 | 4.00 | 2.00 | 2.00 |
| 2 | c | 4.00 | 2.00 | 2.00 | 2.00 |
| 2 | d | 2.00 | 1.00 | 4.00 | 2.00 |
| 3 | a | 2.00 | 2.00 | 2.00 | 4.00 |
| 3 | b | 5.00 | 2.00 | 2.00 | 2.00 |
| 3 | c | 2.00 | 2.00 | 4.00 | 2.00 |
| 3 | d | 2.00 | 5.00 | 2.00 | 2.00 |
| 4 | a | 2.00 | 5.00 | 2.00 | 2.00 |
| 4 | b | 2.00 | 2.00 | 2.00 | 4.00 |
| 4 | c | 2.00 | 2.00 | 5.00 | 2.00 |
| 4 | d | 4.00 | 2.00 | 2.00 | 2.00 |
| 5 | a | 3.50 | 5.00 | 2.50 | 2.50 |
| 5 | b | 3.00 | 2.30 | 5.00 | 2.70 |
| 5 | c | 4.00 | 2.30 | 2.50 | 5.00 |
| 6 | a | 1.00 | 2.00 | 2.00 | 1.00 |
| 6 | b | 3.00 | 1.00 | 1.00 | 1.00 |
| 6 | c | 1.00 | 1.00 | 1.00 | 3.00 |
| 6 | d | 1.00 | 1.00 | 2.00 | 2.00 |
| 6 | e | 2.00 | 3.00 | 1.00 | 1.00 |
| 6 | f | 2.00 | 1.00 | 3.00 | 1.00 |
| 7 | a | 1.00 | 2.00 | 2.00 | 1.00 |
| 7 | b | 2.00 | 1.00 | 3.00 | 1.00 |
| 7 | c | 2.00 | 1.00 | 1.00 | 2.00 |
| 7 | d | 2.00 | 2.00 | 1.00 | 1.00 |
| 7 | e | 2.00 | 1.00 | 1.00 | 3.00 |
| 7 | f | 1.00 | 3.00 | 2.00 | 1.00 |
| 8 | a | 1.00 | 2.00 | 2.00 | 1.00 |
| 8 | b | 2.00 | 1.00 | 1.00 | 2.00 |

TABLE S3

*Chosen $\beta_{k,q}$ hyper-parameters for each possible response to each question (q) by house (k).*

## References.

ROWLING, J. K. Pottermore from J.K.Rowling.
